# Supplementary material for: Exact Spike Train Inference Via $\ell_0$ Optimization
Source: arXiv:1703.08644 source file (2017-11-12)
Supplement: Supplementary file 1 [file appendix-v4.tex]

% !TEX root = ms.tex
\appendix
\section{Proof of Propositions}
\label{sec:appendix}

\subsection{Proof of Proposition~\ref{prop:equiv}}

\begin{proof}

The first sentence follows by inspection. To establish the second sentence, we observe that the cost
\begin{align*}
 \D(y_{a:b}) \equiv \underset{ c_t = \gamma c_{t-1}, \; t=a+1,\ldots,b}{\min}
  \left\{  \frac{1}{2} \sum_{t=a}^{b} \left( y_t - c_t \right)^2 \right\}
\end{align*}
can be rewritten by direct substitution of the constraint as
\begin{align*}
 \D(y_{a:b}) =  \underset{ c_a }{\min}
  \left\{  \frac{1}{2} \sum_{t=a}^{b} \left( y_t - \gamma^{t-a}c_a \right)^2 \right\}.
\end{align*}
This is a least squares problem and is minimized at
\begin{align*}
\hat{c}_{a} = \frac{	\sum_{t=a}^{b} y_{t}\gamma^{t-a}}{ \sum_{t=a}^{b} \gamma^{2(t-a)}},
\end{align*}
which implies that
\begin{align*}
\D(y_{a:b}) = \frac{1}{2} \sum_{t=a}^{b} \left( y_t - \gamma^{t-a}\hat{c}_a \right)^2,
\end{align*}
and furthermore that for $a < t \leq b$ the fitted values are $\hat{c}_{t} = \gamma \hat{c}_{t-1}$. Applying this argument to each segment gives the result stated in Proposition~\ref{prop:equiv}.

\end{proof}

\subsection{Proof of Proposition~\ref{prop:segment-soln}}

\begin{proof}
The first equation follows by expanding the square for the final form of $\D(y_{a:b})$ in the proof of Proposition~\ref{prop:equiv}. Given $\D(y_{a:b})$ we can calculate $\D(y_{a:(b+1)})$ in constant time by storing $\sum_{t=a}^{b} \frac{y_{t}^{2}}{2}$, and $\sum_{t=a}^{b} y_{t}\gamma^{t-a}$ and updating each of these sums for the new data point $y_{b+1}$; we use a closed form expression to calculate $\sum_{t=a}^{b+1} \gamma^{2(t-a)}$. With each of these quantities stored, $\D(\cdot)$ and $\C(\cdot)$ are updated in constant time.

\end{proof}

\section{Choosing $\lambda$ and $\gamma$ Through Cross-Validation}
\label{subsec:cv}

Recall that in  \eqref{eq:nonconvex-nopos}, the parameters $\lambda$ and $\gamma$ are unknown. 
The nonnegative parameter $\lambda$  controls the trade-off between the number of estimated spikes and the quality of the estimated calcium fit to the observed fluorescence. The parameter $\gamma, 0<\gamma < 1$, controls the rate of exponential decay of the calcium. 

In principle, we could choose both $\lambda$ and $\gamma$ by performing cross-validation over a two-dimensional grid of $(\lambda,\gamma)$ values \citep{elemstatlearn}.
 However, this approach would be very computationally intensive, because a very fine grid of values for $\gamma$ would need to be used.

Therefore, instead of performing cross-validation on a two-dimensional grid, we perform cross-validation over a one-dimensional grid of $\lambda$ values. For each value of $\lambda$ in this grid, we solve \eqref{eq:cp} on a training set using a candidate value for $\gamma$. Given the resulting set of changepoints, we solve a one-dimensional constrained optimization problem for $\gamma$. We then refit \eqref{eq:cp} with the optimized value of $\gamma$, and then evaluate the mean squared error (MSE) on a hold-out set. Details are provided in Algorithm~\ref{alg:cv}. Note that in the final output of the algorithm, we take the square root of the optimal value of $\gamma$ in order to address the fact that the cross-validation scheme makes use of training and test sets consisting of alternately-spaced timesteps.

\begin{algorithm}[h!]
    \SetKwInOut{Initialize}{Initialize} 
    \SetKwInOut{Output}{Output}
	\Initialize{ Candidate tuning parameter values $\lambda_{1}, \ldots, \lambda_{M}$;  an initial guess $\hat\gamma$ for the rate of exponential decay; a matrix $\text{cvMSE} \in\R^{M \times 2}$ to store the cross-validated MSEs;  and a  matrix $\Gamma\in\R^{M\times2}$ to store the optimal values of $\gamma$.}
	
	\ForEach{\text{fold} in $1,2$}{
	
	Assign odd timesteps to the training set and even timesteps to the test set for the first fold, and vice-versa for the second fold. Note that $\mathrm{card}(y^{\text{train}})=\mathrm{card}(y^{\text{test}})=T/2$.

	\ForEach{$m=1,\ldots,M$ }{

	Solve \eqref{eq:cp} on the  training set $y^{\text{train}}$ with tuning parameter values $\lambda_m$ and $\hat{\gamma}$, in order to obtain an initial estimate of the changepoints $\tau_1,\ldots,\tau_k$. Set $\tau_0=0$ and $\tau_{k+1}=T/2$. \\
	Given the changepoints $\tau_1,\ldots,\tau_k$, compute the value of $\gamma$ that minimizes the training set MSE,
$$\hat{\gamma} =	\argmin{\gamma}{\sum_{j=0}^{k}  
 \D\left(y^{\text{train}}_{(\tau_{j}+1):\tau_{j+1}}\right) } = \argmin{\gamma}{\sum_{j=0}^{k} \underset{c_{t} = \gamma c_{t-1}, t = \tau_{j} + 2, \ldots, \tau_{j+1}}{\min} \left\{ 	\frac12\sum_{t=\tau_{j}+1}^{\tau_{j+1}} (y^{\text{train}}_{t} - c_{t})^{2}	\right\}}.$$
 This can be done via numerical optimization. Set $\Gamma_{m, \text{fold}} = \hat\gamma$.\\
	Solve \eqref{eq:cp} on the training set $y^{\text{train}}$ with tuning parameter values $\lambda_m$ and $\hat{\gamma}$ in order to obtain fitted values $\hat{c}^{\text{train}}$.\\
Average adjacent fitted values in order to obtain predictions on the test set $y^{\text{test}}$,
	\begin{align*}
		\hat{c}^{\text{test}} &= \frac{\hat{c}^{\text{train}}_{1:(T/2-1)} + \hat{c}^{\text{train}}_{2:(T/2)}}{2}.
	\end{align*}\\
	Calculate and store the test set MSE,
	\begin{align*}
		\text{cvMSE}_{m, \text{fold}} &= \frac{2}{T} \sum_{t = 1}^{T/2} \left( y^{\text{test}}_{t} - \hat{c}_{t}^{\text{test}}\right)^{2}.
	\end{align*}
	\\ 
	}}
	
	Average the test set MSE and $\Gamma$ over folds,
	\begin{align*}
	\overline{\text{cvMSE}}_{m} =  \frac12 \left( \text{cvMSE}_{m, 1} + \text{cvMSE}_{m, 2} \right), \quad
	\overline{\Gamma}_{m} =  \frac12 \left( \Gamma_{m, 1} + \Gamma_{m, 2} \right), \mbox{ for } m=1,\ldots,M.
	\end{align*}\\
	Calculate $\hat{m} = \argmin{m}{\overline{\text{cvMSE}}_{m}}$.\\
	Calculate the standard error of the test set MSE over folds,
	\begin{align*}
	\text{se}\left({\text{cvMSE}}\right)_{m} &= \sqrt{\frac{\left( \text{cvMSE}_{m, 1} - 	\overline{\text{cvMSE}}_{m}	\right)^{2} + \left( \text{cvMSE}_{m, 2} - 	\overline{\text{cvMSE}}_{m}	\right)^{2}}{2}}, \mbox{ for } m=1,\ldots,M.
	\end{align*}\\
	Calculate $$m^* = \max\left\{m: \overline{\text{cvMSE}}_{m} \leq \overline{\text{cvMSE}}_{\hat{m}} + \text{se}\left({\text{cvMSE}}\right)_{\hat{m}}\right\}.$$

	\Output{The values
	 $\left(\lambda_{\hat{m}},\sqrt{\overline{\Gamma}_{\hat{m}}}  \right)$ that 
	minimize the cross-validated MSE, and the values 
	$\left(\lambda_{m^*},\sqrt{\overline{\Gamma}_{m^*}  } \right)$ selected 
	based on the one-standard-error rule \citep{elemstatlearn}.}
    \caption{A Cross-Validation Scheme for Choosing $\lambda$ and $\gamma$ in \eqref{eq:nonconvex-nopos}}\label{alg:cv}
\end{algorithm}

\clearpage
\section{Heuristic Approaches}
\label{sec:heur}
%Numerical examples where the objective achieved by J2 (w smin chosen automatically) is higher than L0 
%Display figures where J2 w smin is chosen automatically does badly? 
%Display figures where post thresholding for a range of threshold values
%we claim that this is sensitive to choice of threshold and is not elegant 
%l0 is more elegant and at least as good as the hacks

In this section, we explore two heuristic approaches that encourage further spike sparsity: post-thresholding and a non-convex modification of \eqref{eq:convex-fried} proposed by \cite {friedrichfast2017}. Performance is shown for a range of tuning parameters on a subset of the \cite{chen2013ultrasensitive} data presented in Section~\ref{subsec:chen}. 

Post-thresholding is a simple intuitive way to induce additional sparsity to the solution of \eqref{eq:convex-fried}. Given a threshold $L$ and solution $\hat{s}_{2}, \ldots, \hat{s}_{T}$ of the $\ell_{1}$ problem \eqref{eq:convex-fried}, the post-thresholding solution is $\tilde{s}_{t} = \hat{s}_{t} 1_{(\hat{s}_{t} \geq L)}$ for $t = 2, \ldots, T$. 

Figure~\ref{fig:threshold} illustrates the behavior of the post-thresholding method for different thresholds $L$, $\lambda = 1$, and $\gamma = 0.9864405$. As $L$ increases from $10^{-8}$ to $0.1$, in panels (a) to (b), the post-thresholding solution is very close to the ground truth between $10-30$s; however the zoomed in view, in panels (d) and (e), show that with $L = 0.1$ spikes are overestimated between $6-8$s. Increasing $L$ to $0.12$, in panels (c) and (f), induces additional sparsity, but causes several missed spikes between $20-25$s. 

\cite {friedrichfast2017} consider a variant of the optimization problem \eqref{eq:convex-fried}

\begin{equation}
\minimize{c_1,\ldots,c_T, s_2,\ldots,s_T}{  \frac{1}{2} \sum_{t=1}^T \left( y_t - c_t \right)^2} \mbox{ subject to } s_t = c_t - \gamma c_{t-1} \geq s_{min} \mbox{ or } s_{t} = 0,
   \label{eq:nonconvex-smin}
   \end{equation}
obtained from \eqref{eq:convex-fried} by setting $\lambda = 0$ and changing the convex positivity constraint to the non-convex constraint 
$s_t = c_t - \gamma c_{t-1} \geq s_{min} \mbox{ or } s_{t} = 0$. 

Figure~\ref{fig:threshold} illustrates the behavior of this variant applied to the same data as Figure~\ref{fig:threshold} for different $s_{min}$, and $\gamma = 0.9864405$. As $s_{min}$ increases from $10^{-8}$ to $0.1$, in panels (a) to (b), spikes are still overestimated, but as $s_{min}$ increases to $0.3$, in panel (c), the solution to \eqref{eq:nonconvex-smin} is very similar to the solution of \eqref{eq:nonconvex-nopos} with $\lambda = 0.6$ as well as the ground truth spikes. 

It is important to note that the modification \eqref{eq:nonconvex-smin} results in a non-convex problem. Furthermore, the algorithm of \cite {friedrichfast2017} to solve \eqref{eq:nonconvex-smin} is not guaranteed to find the global minimum. For example, on the \citet{chen2013ultrasensitive} data in Figure~\ref{fig:smin}, the $\ell_{0}$ solution with $\lambda = 0.6$ is feasible for the problem \eqref{eq:nonconvex-smin} with $s_{min} = 0.3$ and has objective value $7.86$, whereas the approximate solution from \cite {friedrichfast2017} has objective value $8.57$. We emphasize that this is quite remarkable because the $\ell_{0}$ problem \eqref{eq:nonconvex-nopos} solves a completely different optimization problem yet is still feasible and obtains a lower objective than the solution given by the algorithm of \cite {friedrichfast2017} for problem \eqref{eq:nonconvex-smin}. 

Both of these modifications to the $\ell_{1}$ problem \eqref{eq:convex-fried} attempt to solve \eqref{eq:nonconvex-pis1}. However, post-thresholding is a heuristic that relies on an additional tuning parameter, and \eqref{eq:nonconvex-smin} is an approximation without global guarantees. Figure~\ref{fig:threshold} provides evidence that while thresholding does a good job it overestimates spikes. On the other hand, Figure~\ref{fig:smin} depicts great empirical performance for the approximate solution of \eqref{eq:nonconvex-smin}. Unfortunately the greedy algorithm of \cite {friedrichfast2017} does not typically achieve the global optimum. In contrast to both of these proposals, the $\ell_{0}$ procedure of this paper is an elegant approach that exactly solves a slight modification of \eqref{eq:nonconvex-pis1} efficiently.

\begin{landscape}

\begin{figure}
\centering
\begin{subfigure}[b]{0.4\textheight}
\centering
\includegraphics[scale=.5]{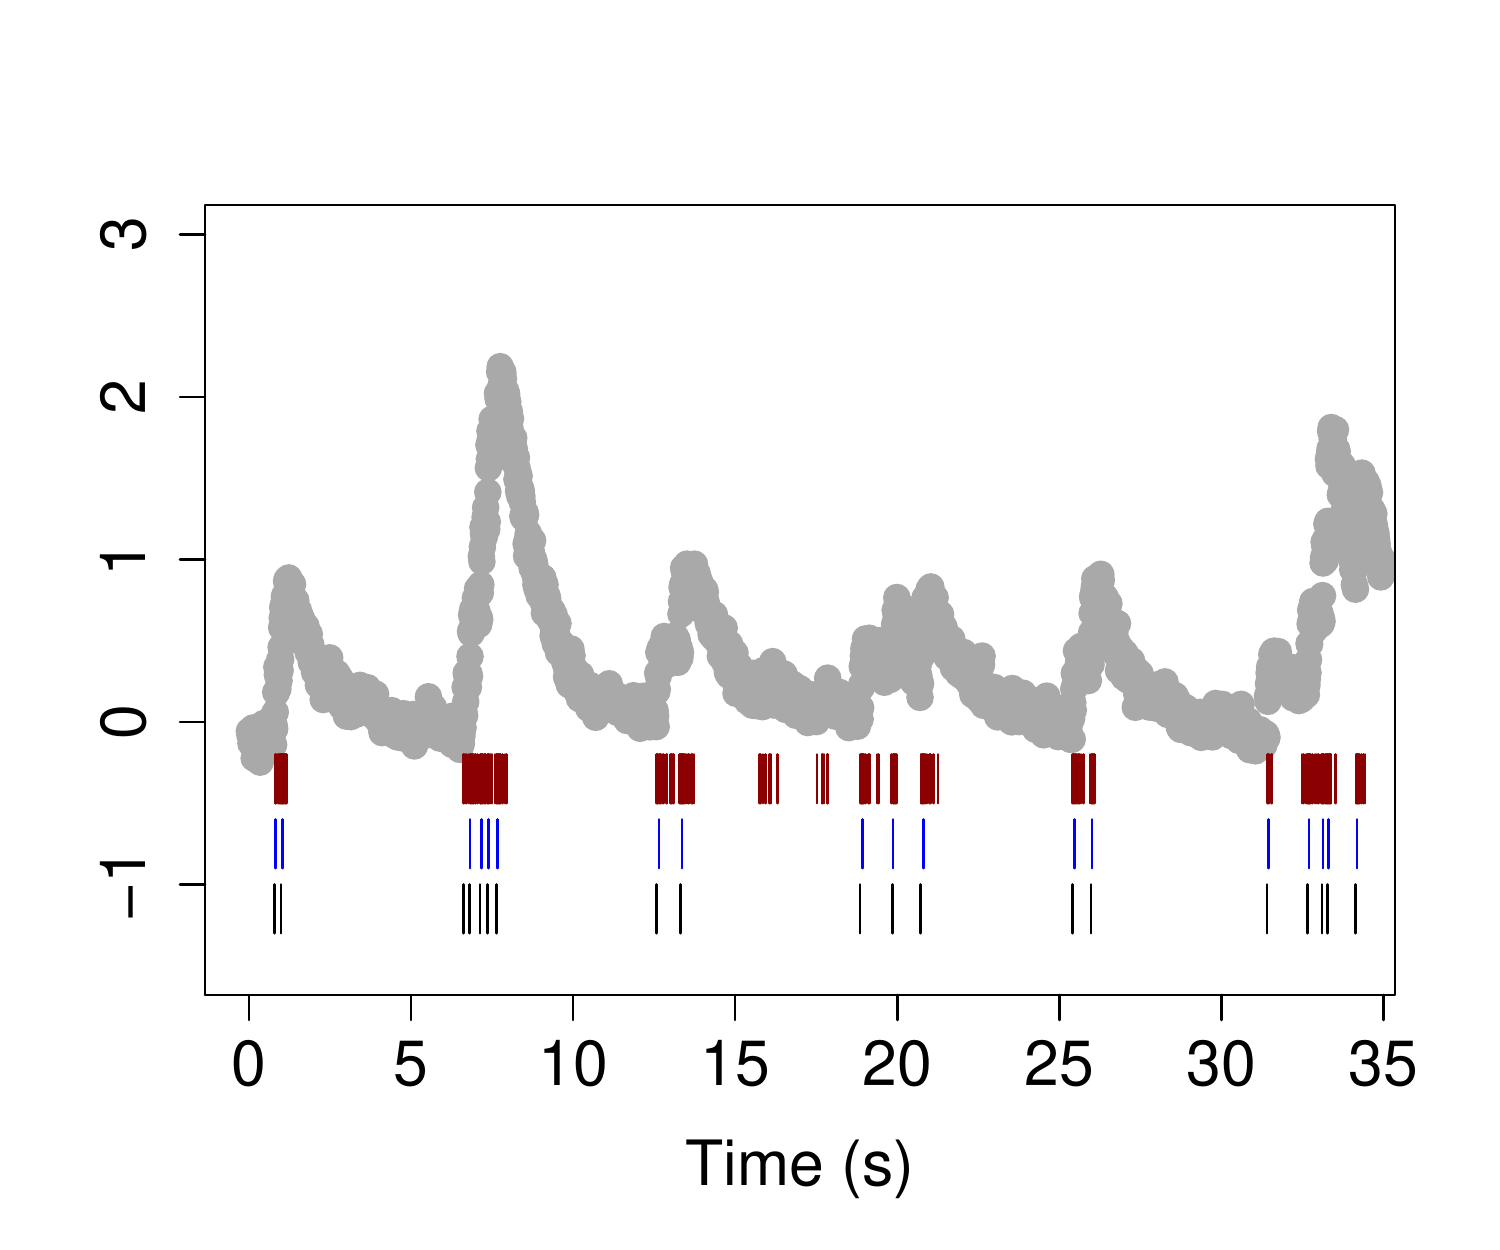} 
\caption{$L = 10^{-8}$.}
\end{subfigure}
\begin{subfigure}[b]{0.4\textheight}
\centering
\includegraphics[scale=.5]{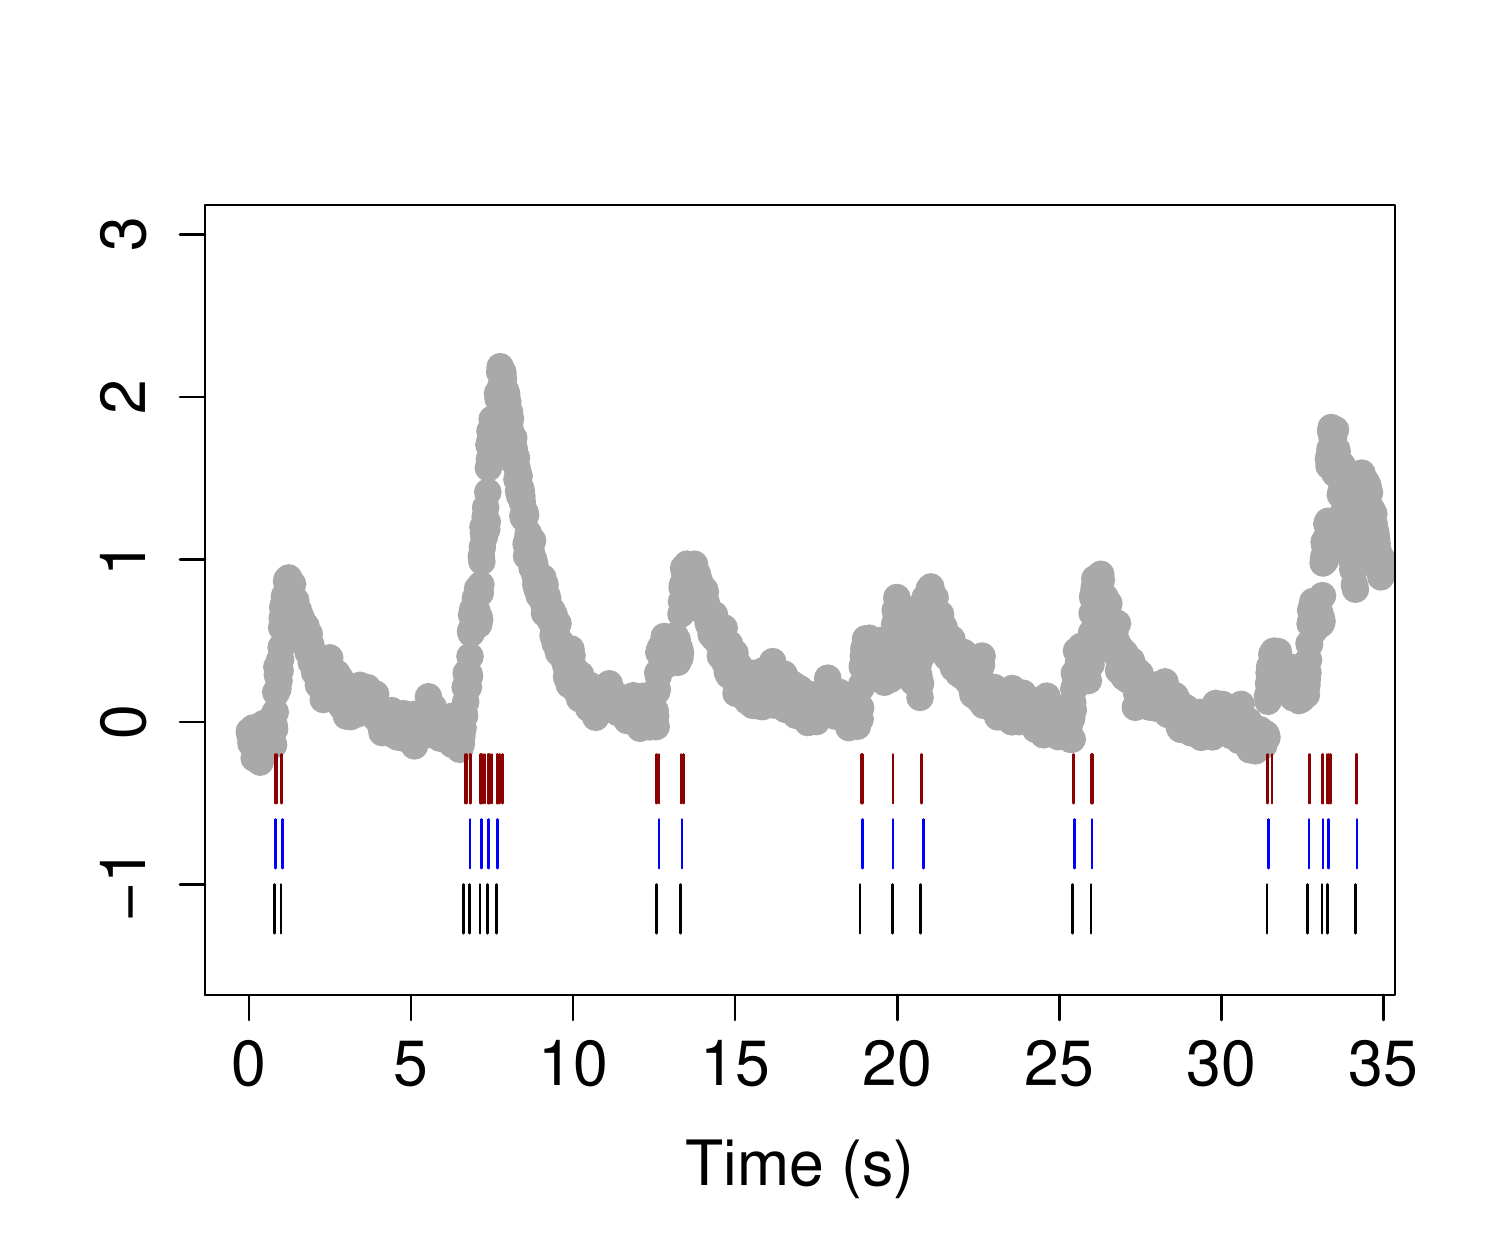} 
\caption{$L = 0.1$.}
\end{subfigure}
\begin{subfigure}[b]{0.4\textheight}
\centering
\includegraphics[scale=.5]{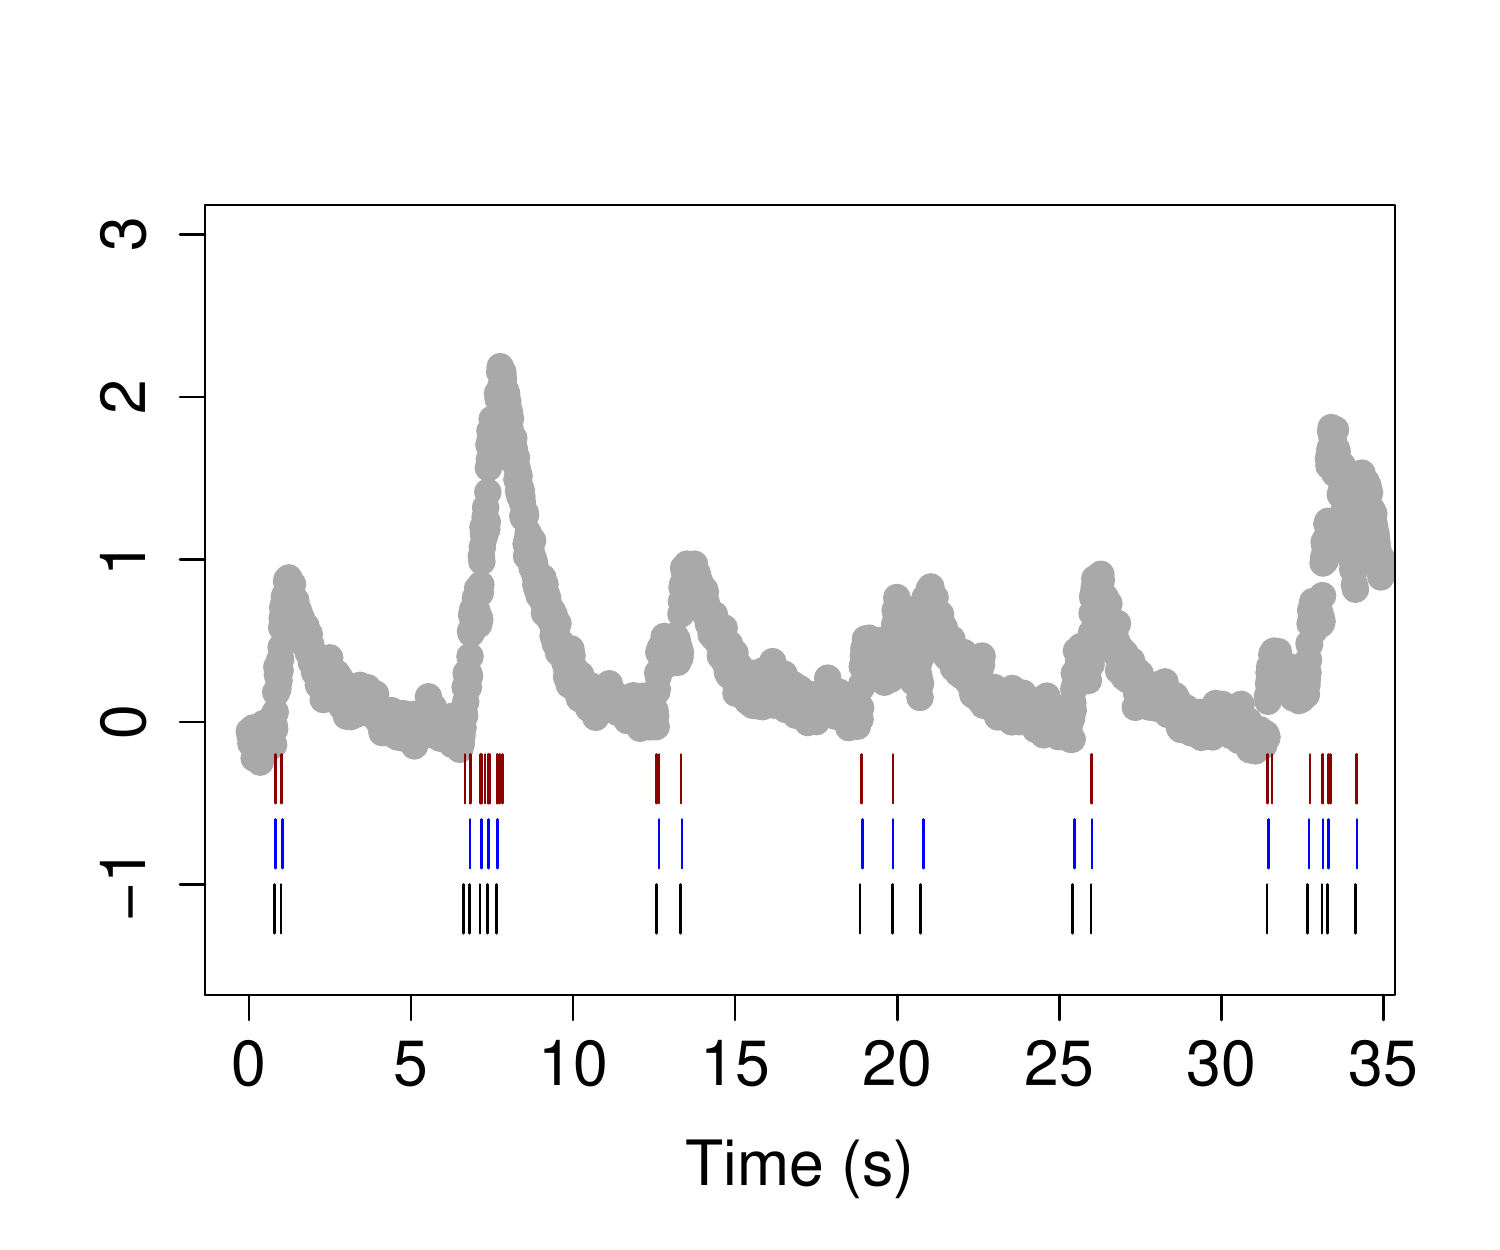}  
\caption{$L = 0.12$.}
\end{subfigure}%

\begin{subfigure}[b]{0.4\textheight}
\centering
\includegraphics[scale=.5]{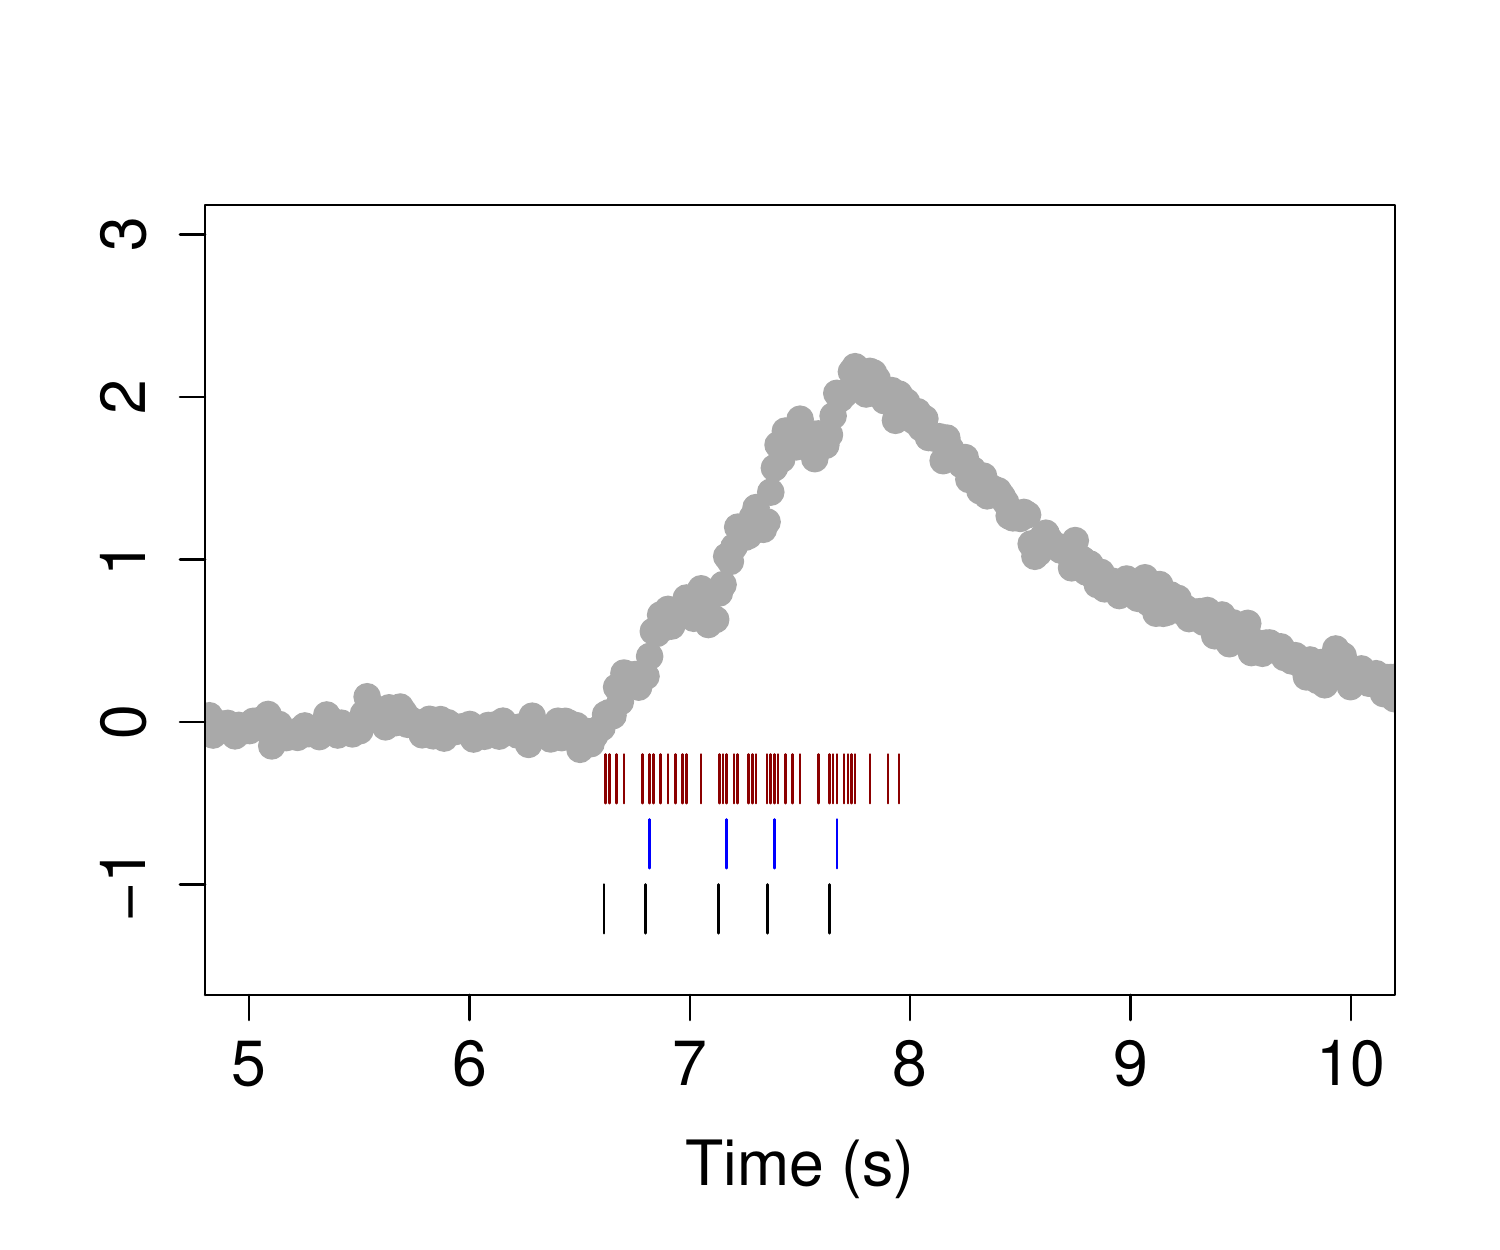} 
\caption{Zoomed $L = 10^{-8}$.}
\end{subfigure}
\begin{subfigure}[b]{0.4\textheight}
\centering
\includegraphics[scale=.5]{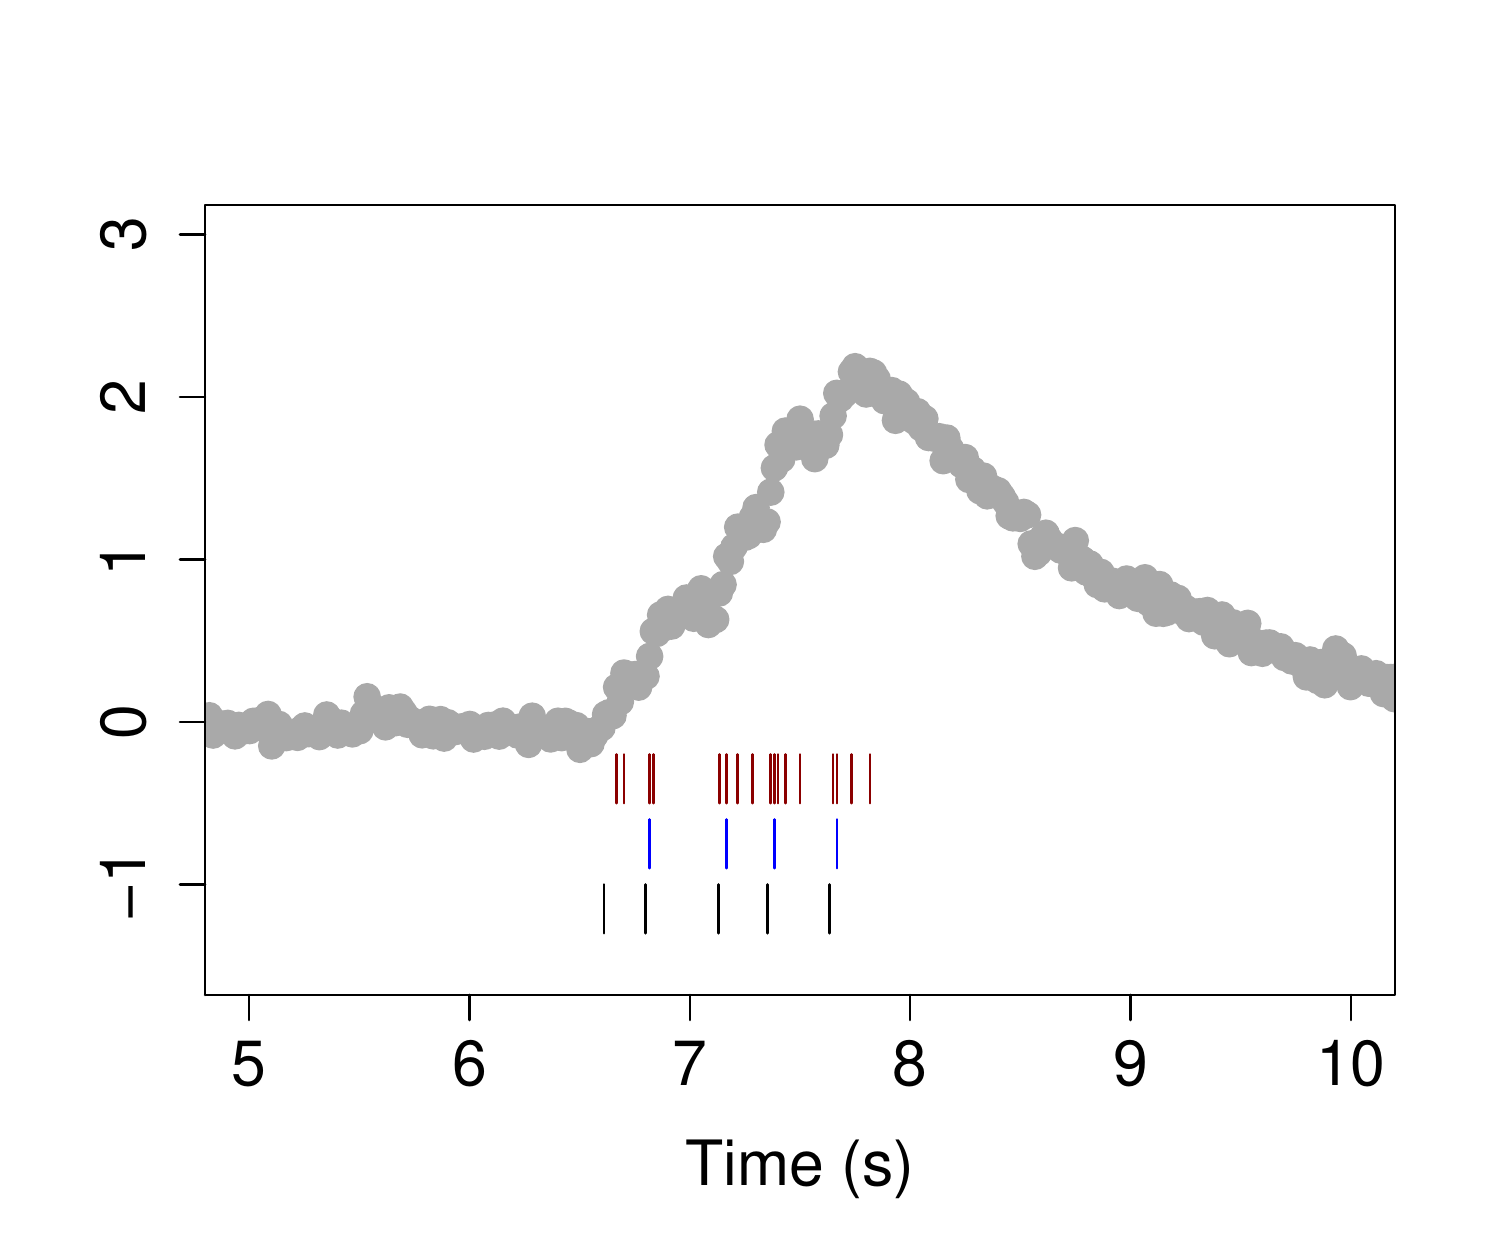} 
\caption{Zoomed $L = 0.1$.}
\end{subfigure}
\begin{subfigure}[b]{0.4\textheight}
\centering
\includegraphics[scale=.5]{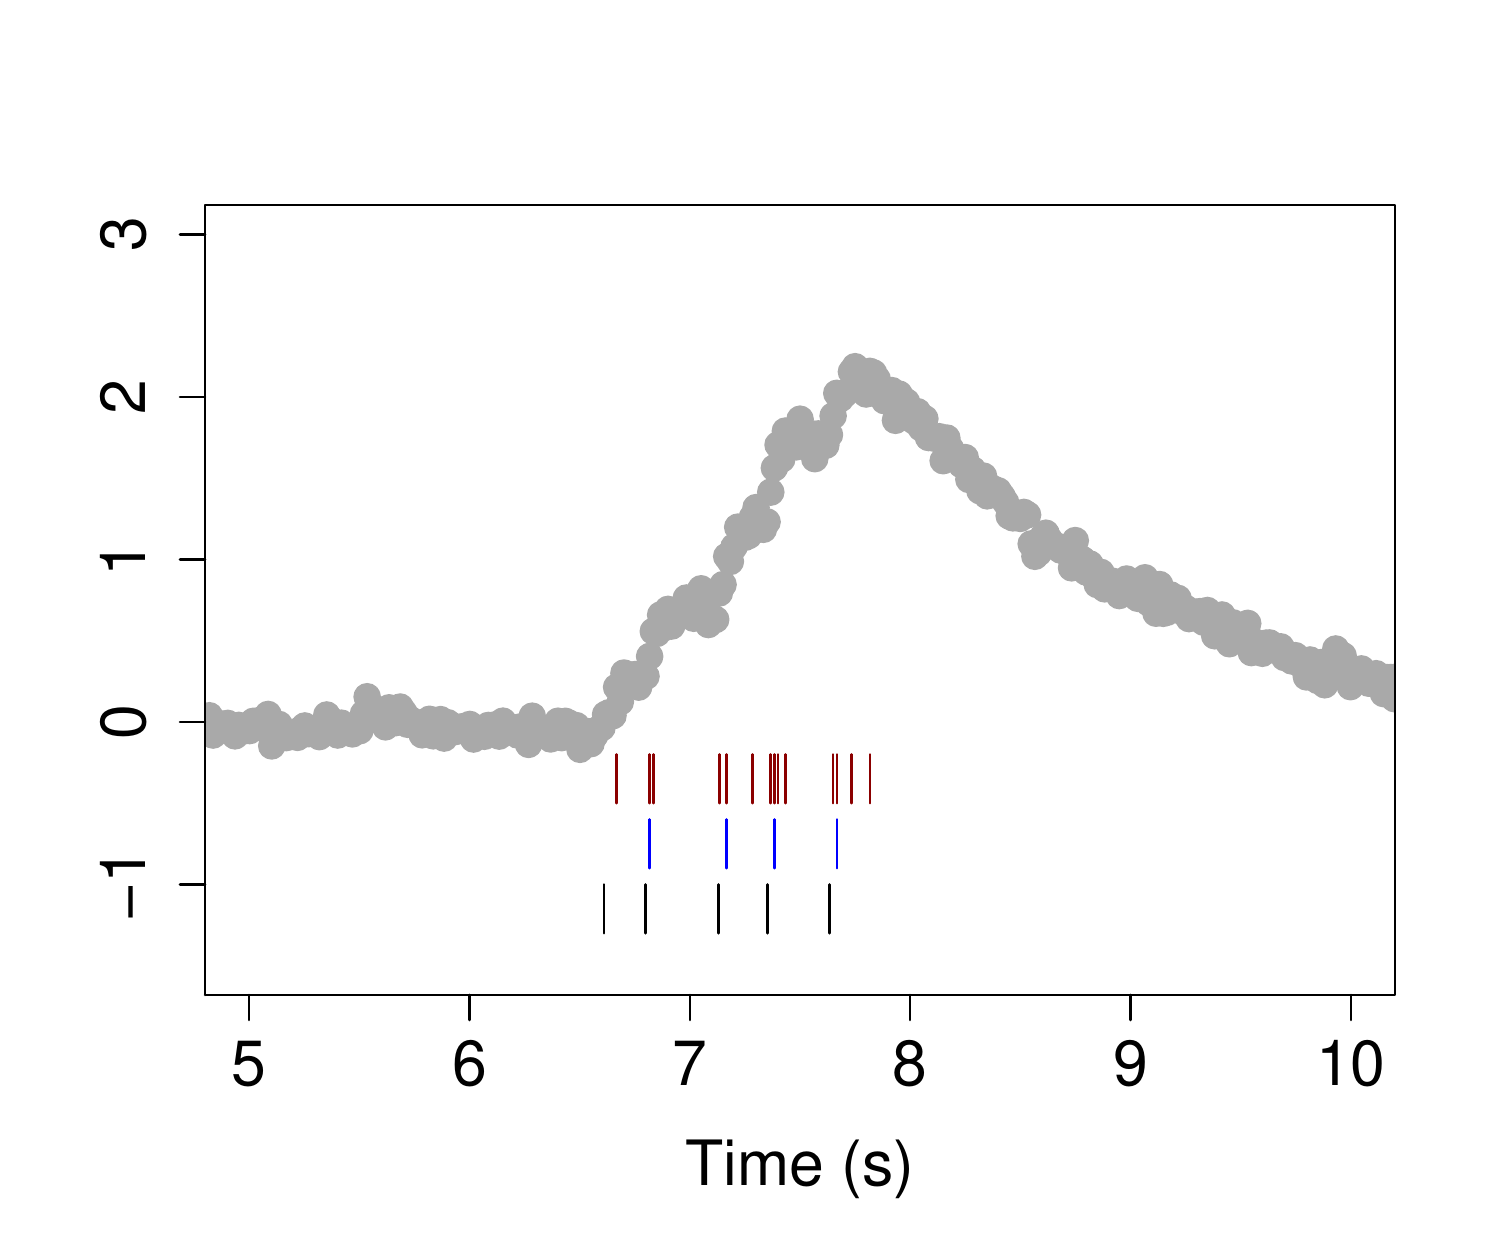} 
\caption{Zoomed $L = 0.12$.}
\end{subfigure}

\caption{ Spike detection for  cell 2002 of the \citet{chen2013ultrasensitive} data. In each panel, the observed fluorescence (\protect\includegraphics[height=0.4em]{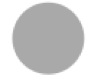}) and true spikes (\protect\includegraphics[height=0.3em]{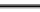}) are displayed. Estimated  spikes $\tilde{s}_{t}$ from post-thresholding are shown in (\protect\includegraphics[height=0.4em]{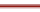}), and the estimated spikes from the $\ell_{0}$ problem \eqref{eq:nonconvex-nopos} with $\lambda = 0.6$ are shown in (\protect\includegraphics[height=0.4em]{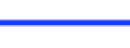}). Times $0s-35s$ are shown in the top row; the second row zooms into time $5s-10s$ to illustrate behavior around a large increase in calcium concentration. Columns correspond to different thresholds $L$.}
\label{fig:threshold}
\end{figure}

\begin{figure}
\centering
\begin{subfigure}[b]{0.4\textheight}
\centering
\includegraphics[scale=.5]{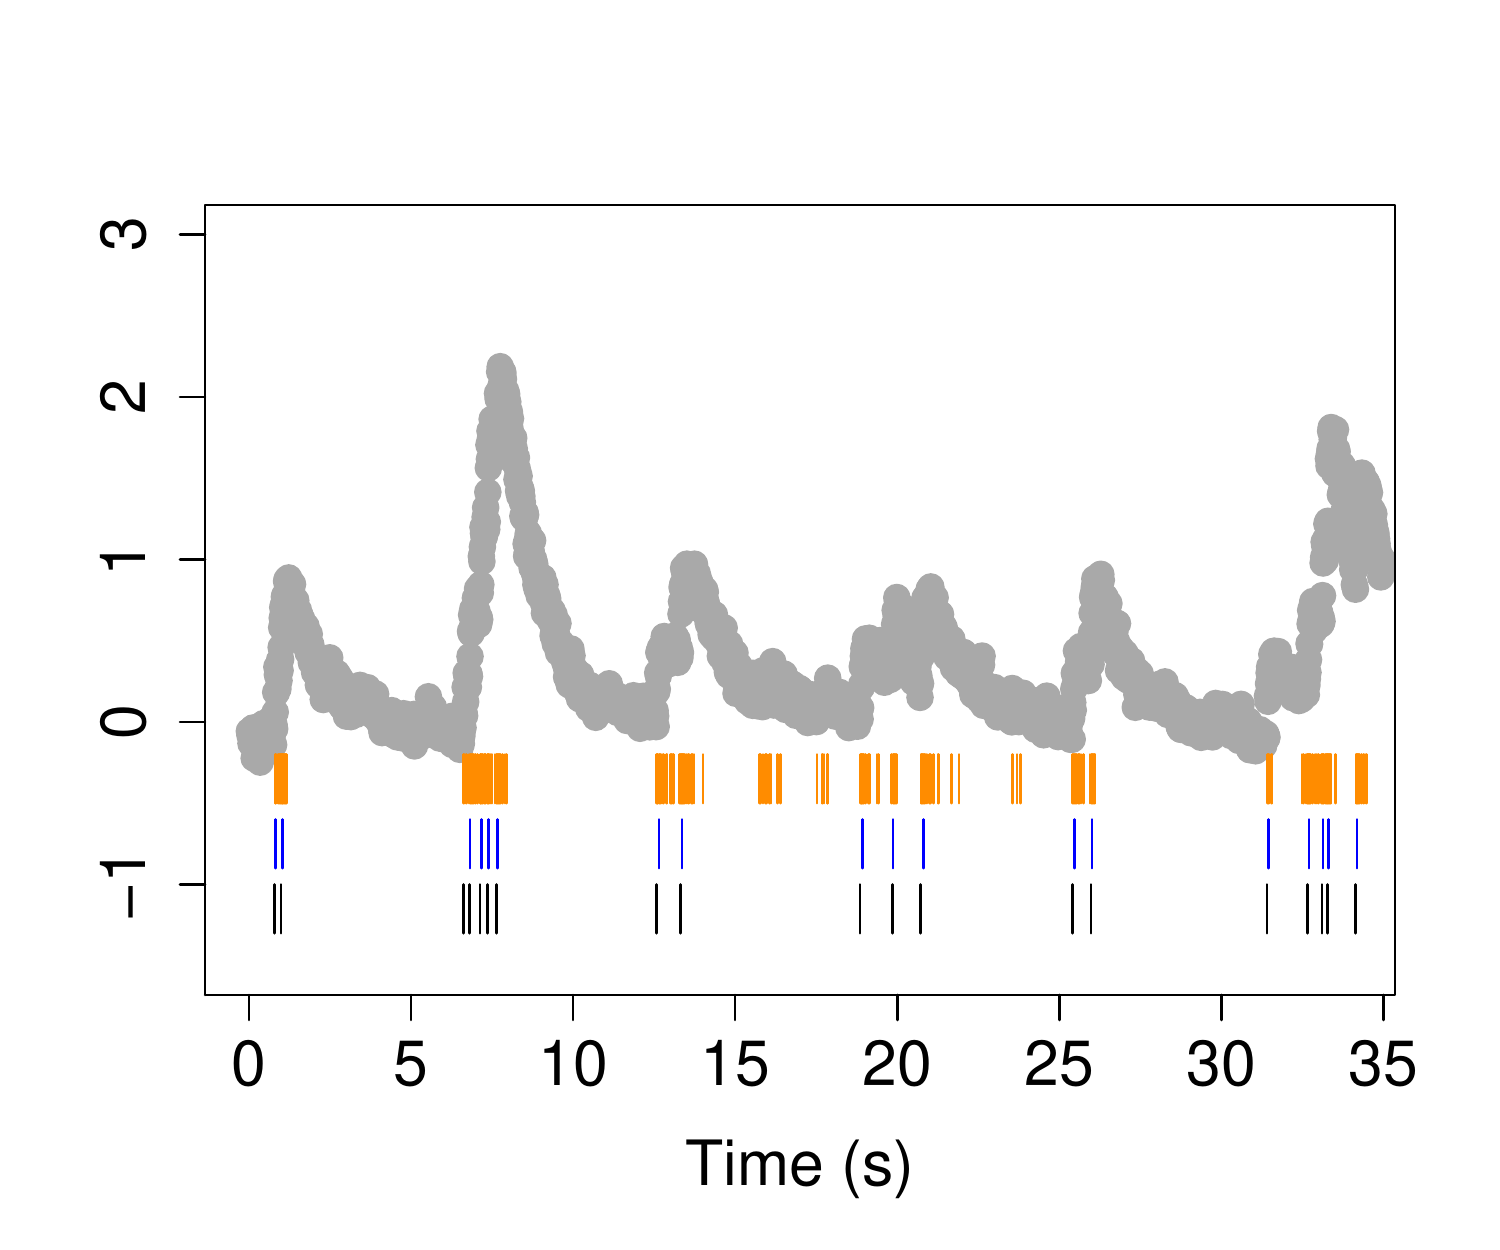} 
\caption{$s_{min} = 10^{-8}$.}
\end{subfigure}
\begin{subfigure}[b]{0.4\textheight}
\centering
\includegraphics[scale=.5]{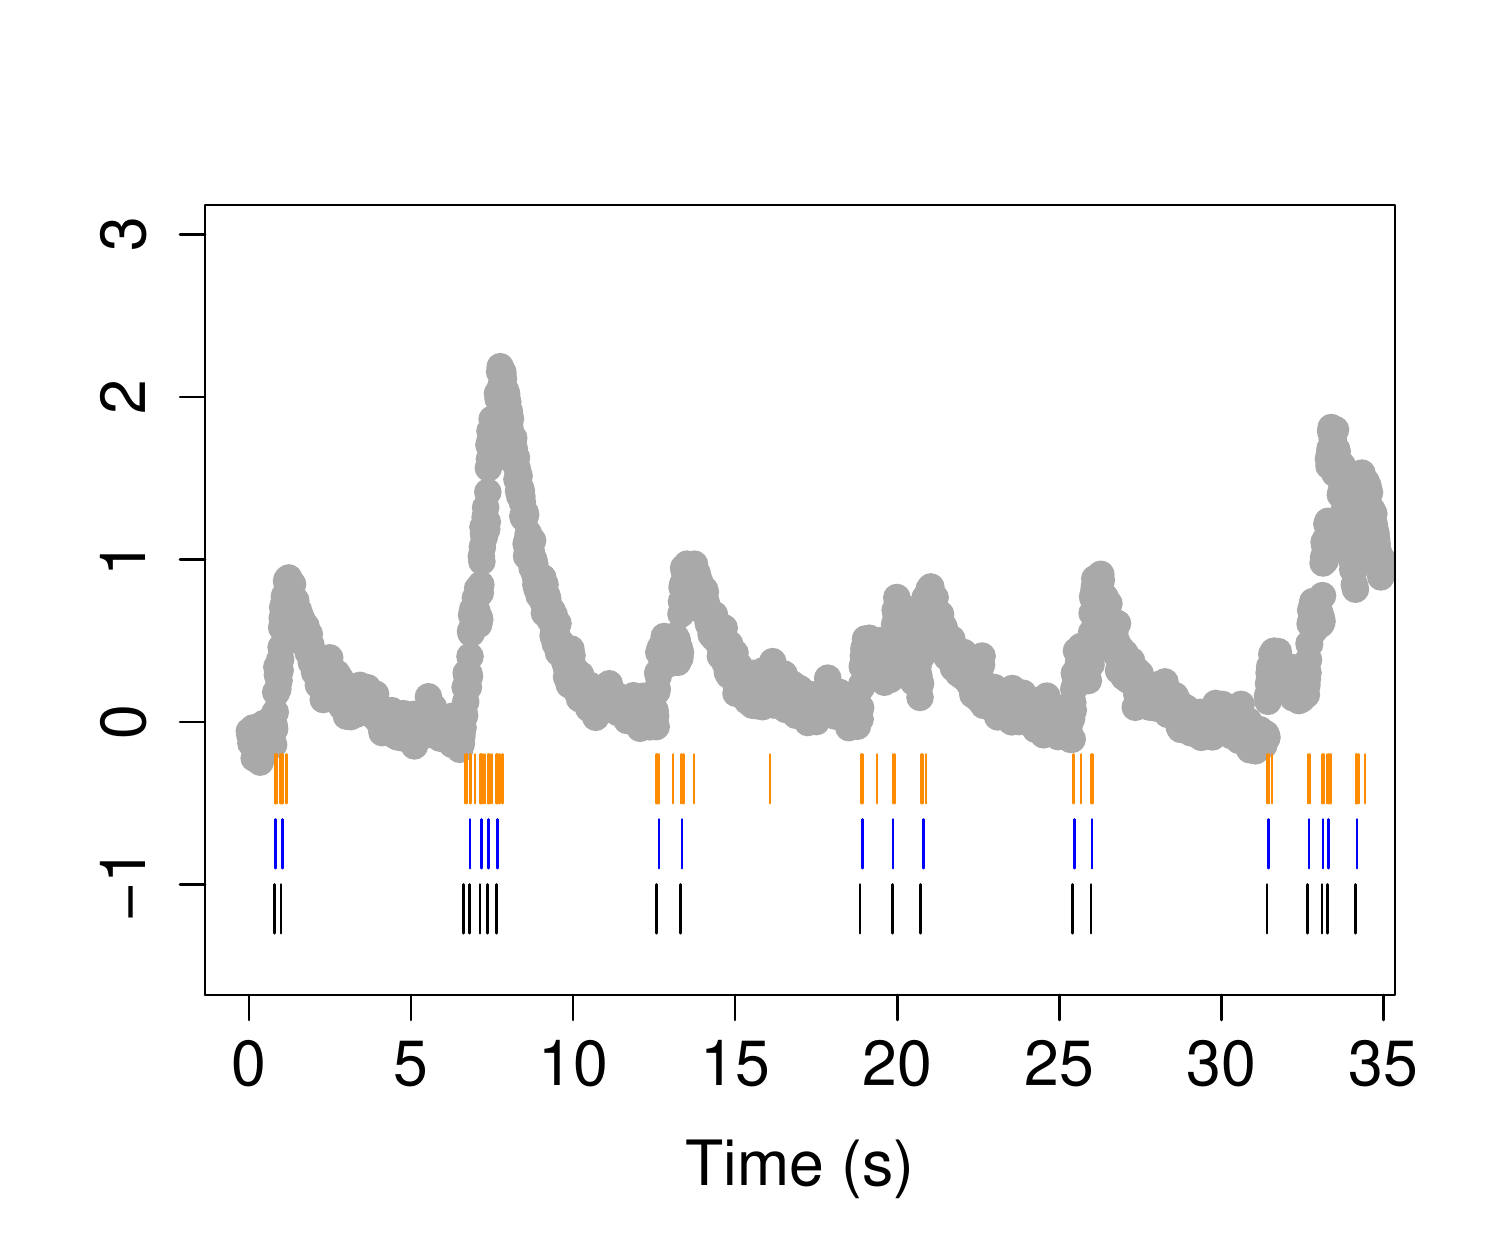} 
\caption{$s_{min} = 0.1$.}
\end{subfigure}
\begin{subfigure}[b]{0.4\textheight}
\centering
\includegraphics[scale=.5]{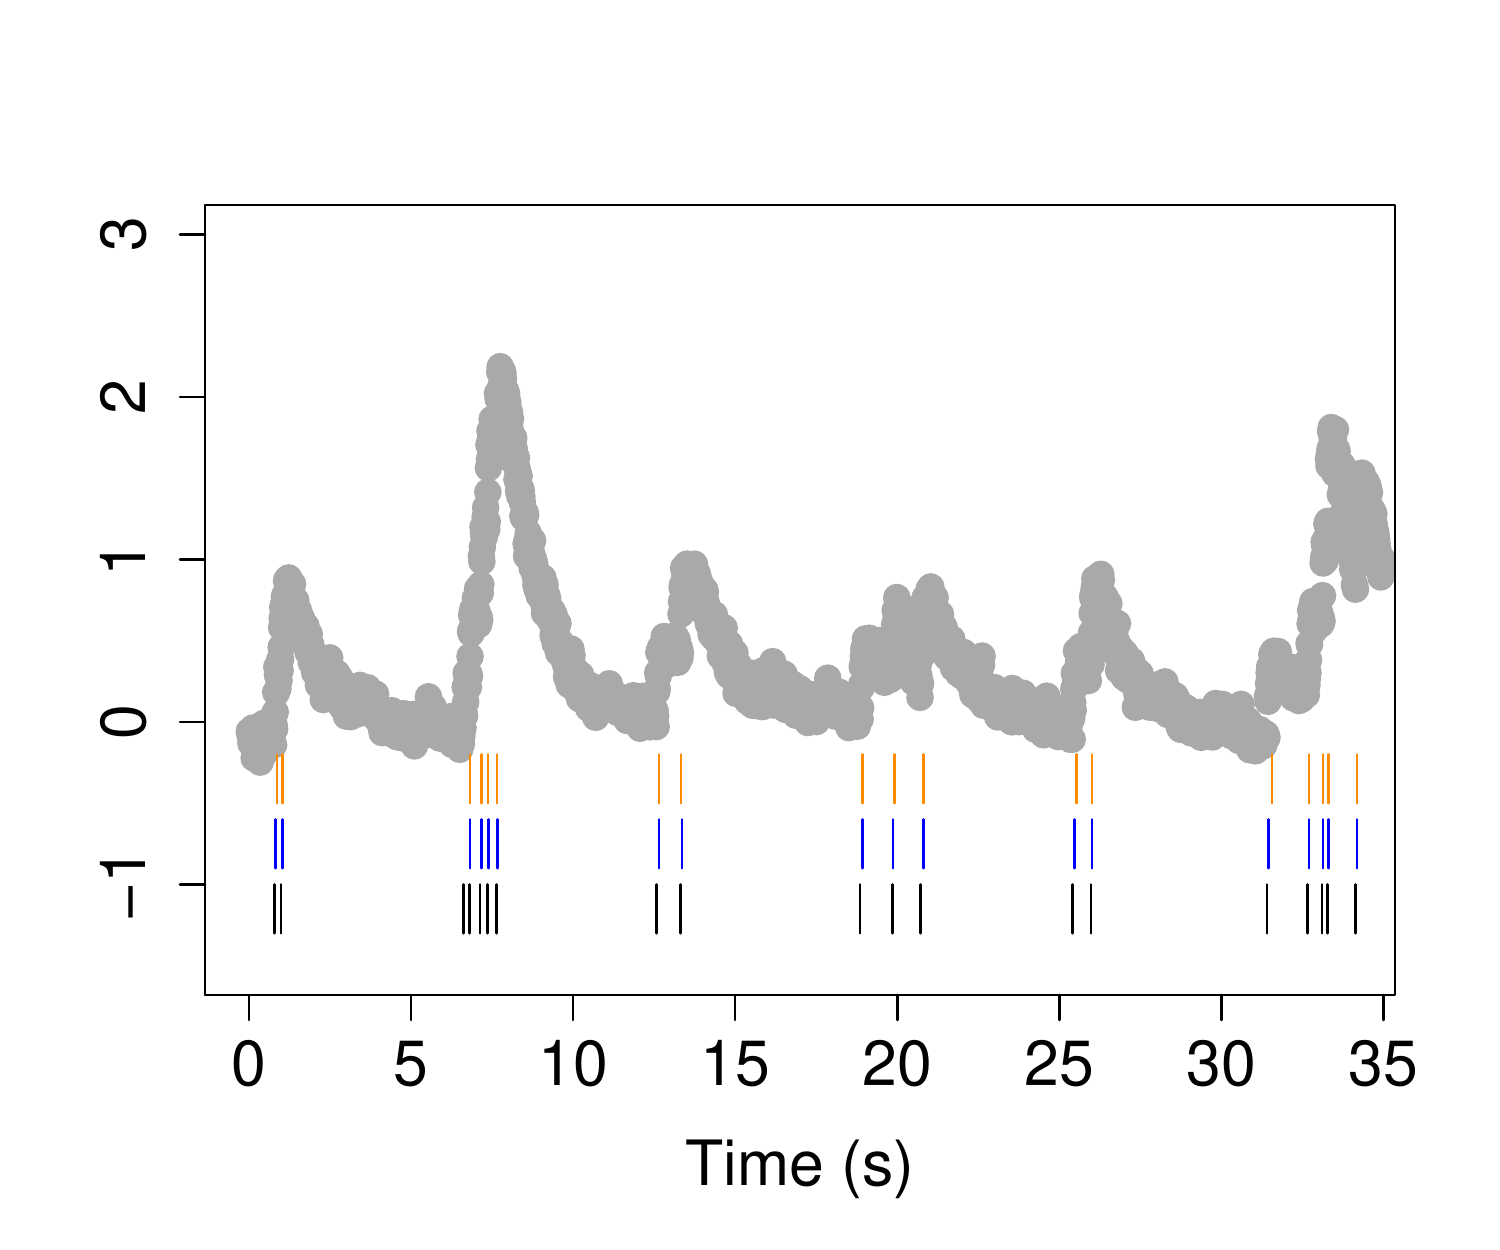}  
\caption{$s_{min} = 0.3$.}
\end{subfigure}%

\begin{subfigure}[b]{0.4\textheight}
\centering
\includegraphics[scale=.5]{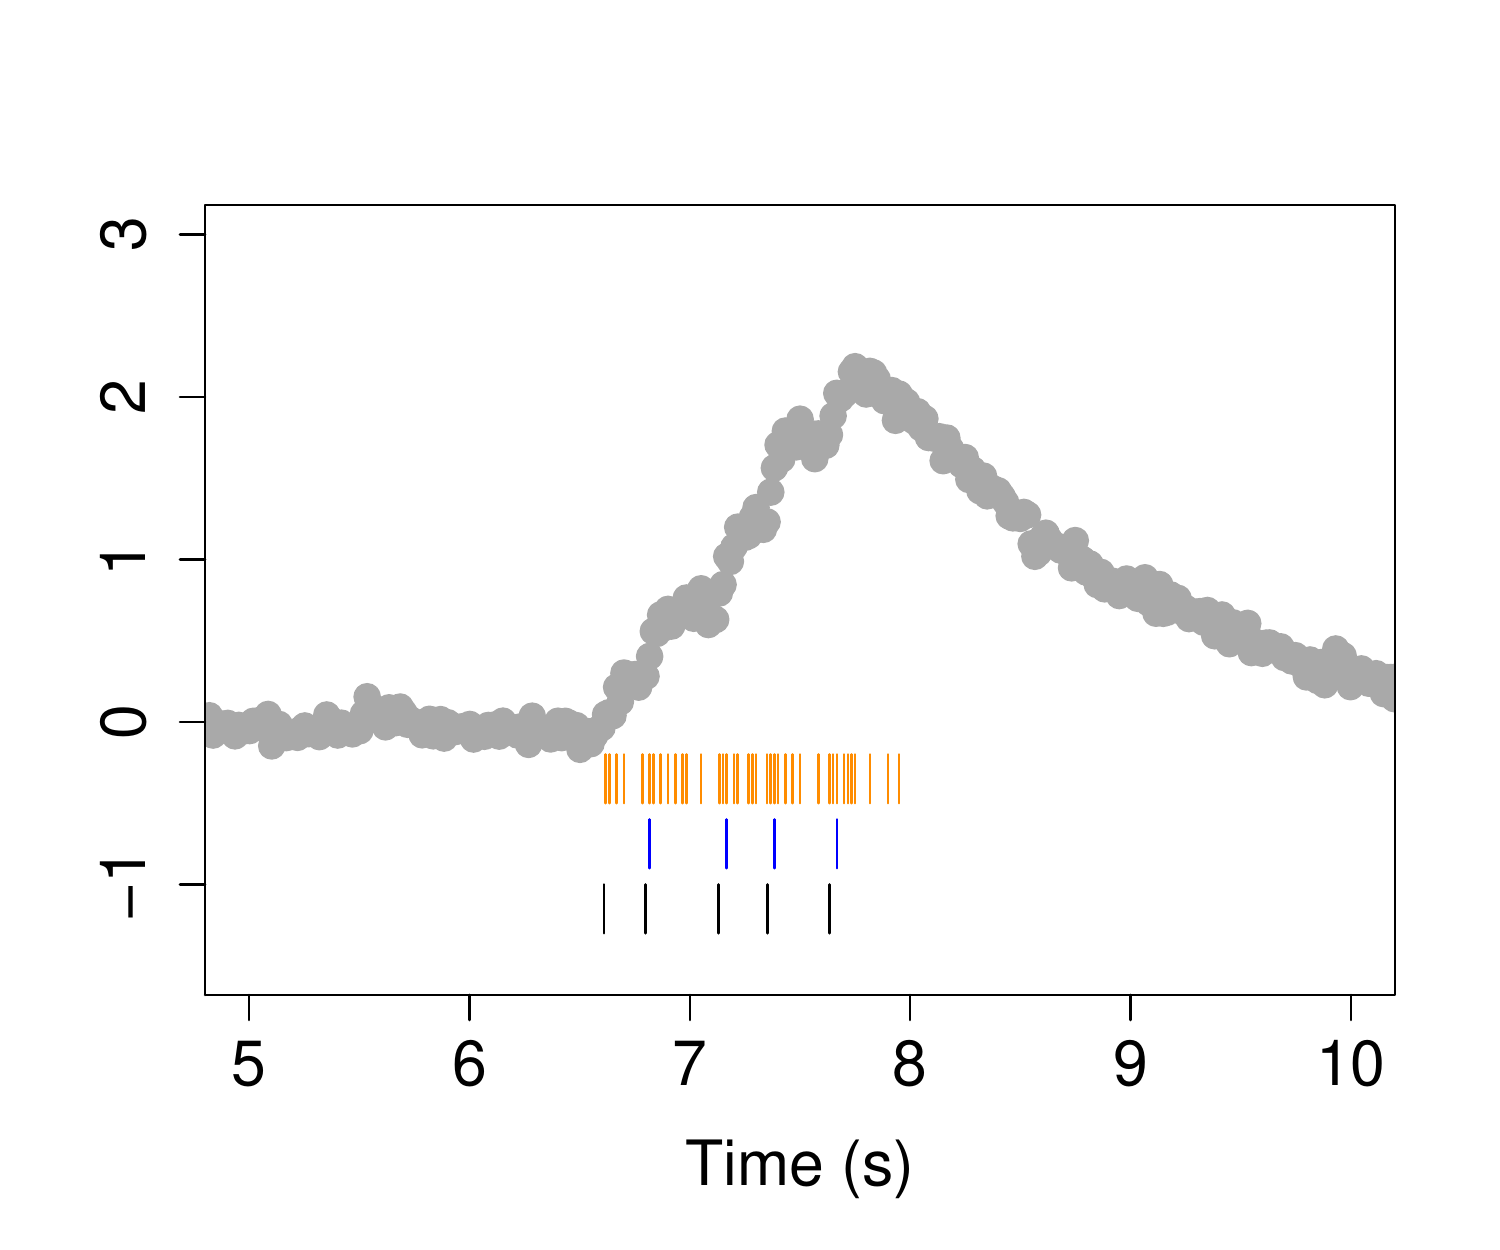} 
\caption{Zoomed $s_{min} = 10^{-8}$.}
\end{subfigure}
\begin{subfigure}[b]{0.4\textheight}
\centering
\includegraphics[scale=.5]{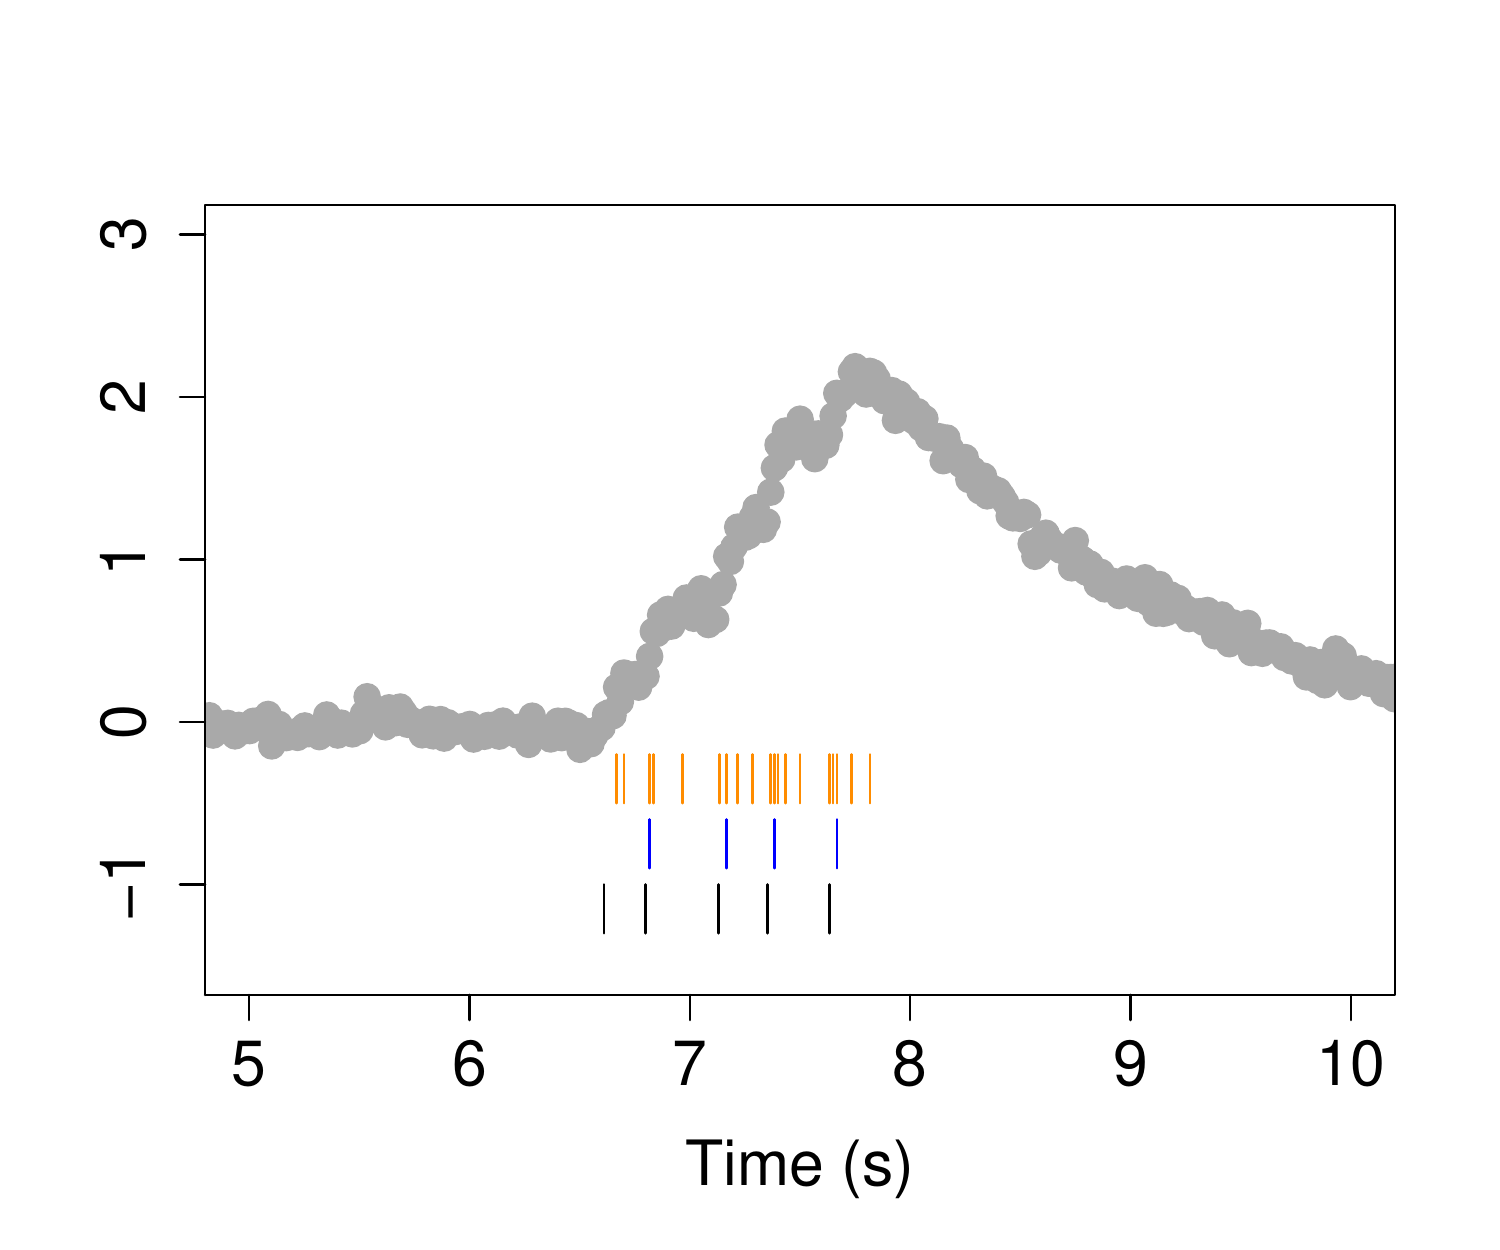} 
\caption{Zoomed $s_{min} = 0.1$.}
\end{subfigure}
\begin{subfigure}[b]{0.4\textheight}
\centering
\includegraphics[scale=.5]{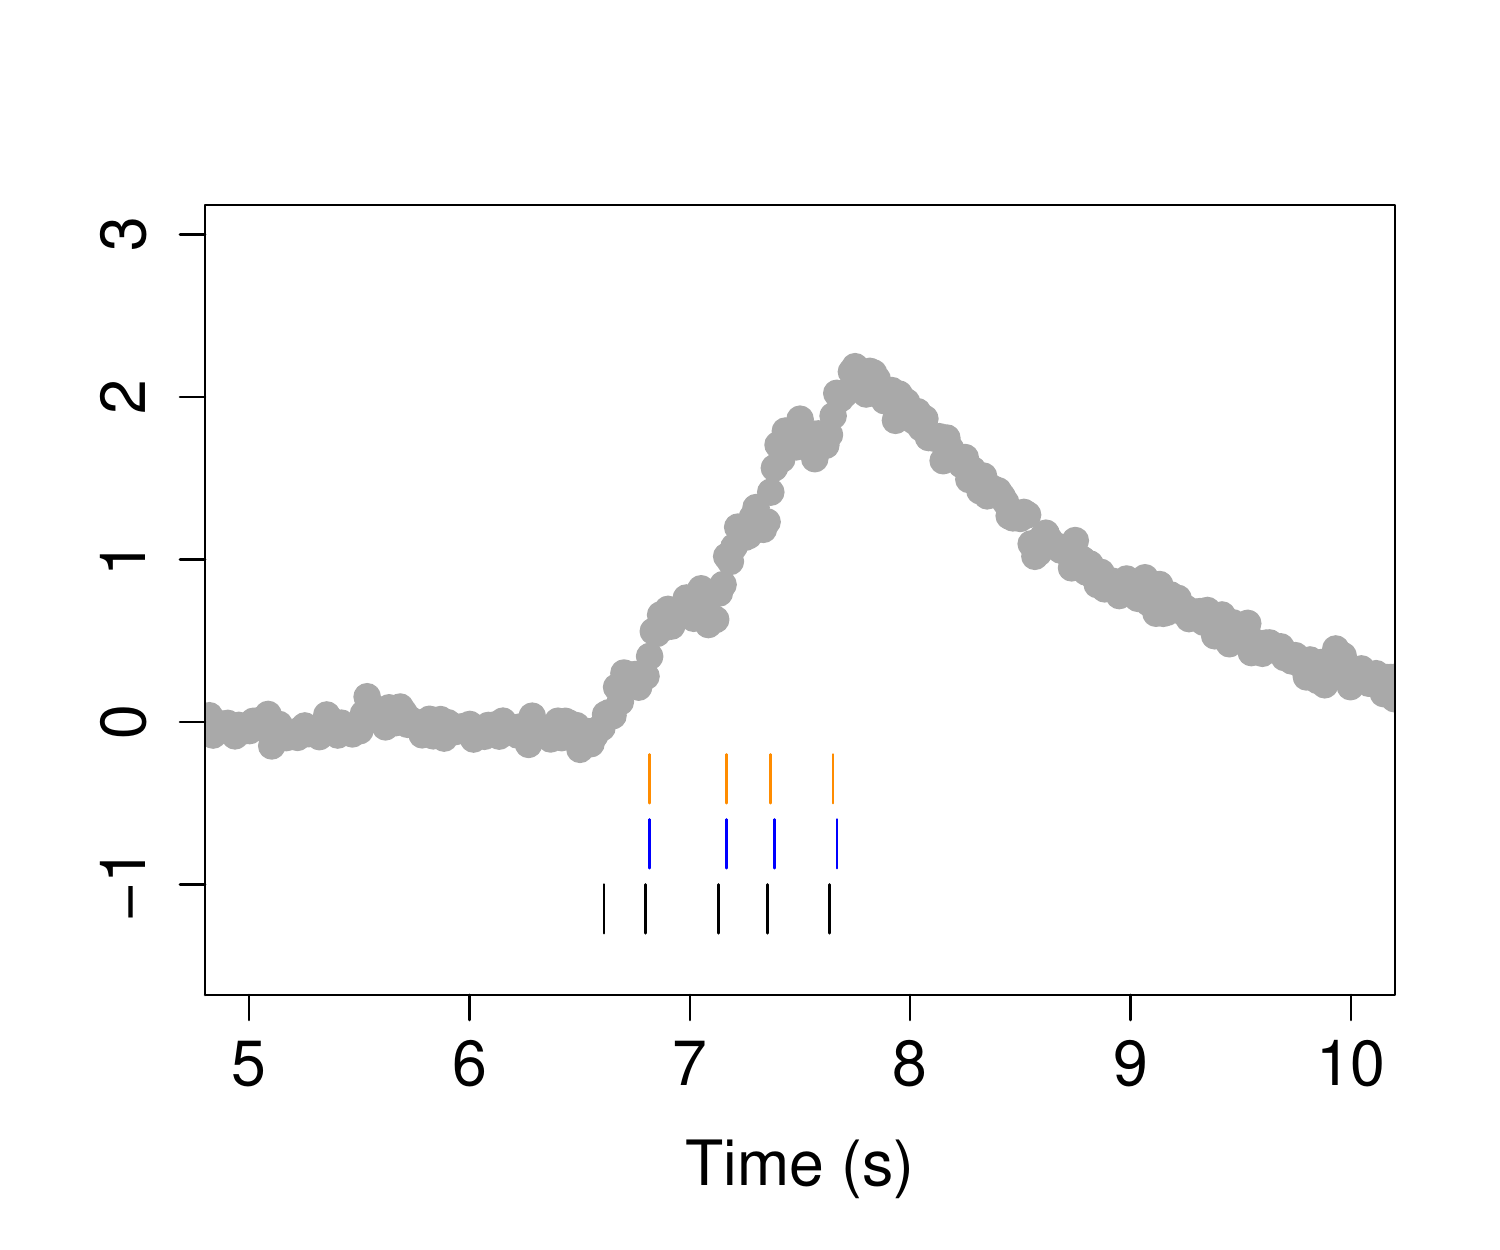} 
\caption{Zoomed $s_{min} = 0.3$.}
\end{subfigure}
\caption{Spike detection for  cell 2002 of the \citet{chen2013ultrasensitive} data. In each panel, the observed fluorescence (\protect\includegraphics[height=0.4em]{grey-circle}) and true spikes (\protect\includegraphics[height=0.3em]{black}) are displayed. Estimated  spikes from problem \eqref{eq:nonconvex-smin} are shown in (\protect\includegraphics[height=0.3em]{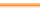}), and the estimated spikes from the $\ell_{0}$ problem \eqref{eq:nonconvex-nopos} with $\lambda = 0.6$ are shown in (\protect\includegraphics[height=0.4em]{blue}). Times $0s-35s$ are shown in the top row; the second row zooms into time $5s-10s$ to illustrate behavior around a large increase in calcium concentration. Columns correspond to different values of $s_{min}$. 
}
\label{fig:smin}
\end{figure}
\end{landscape}

\clearpage
